# Supplementary material for: Difference-frequency generation in an AlGaAs Bragg-reflection waveguide using an on-chip electrically-pumped quantum dot laser
Source: arXiv:2101.08097 ancillary file (2022-02-07)
Supplement: Supplementary file 1 [file 2021_DFG_Suppl.pdf]

# Supplementary Material: Difference-frequency generation in an AlGaAs Bragg-reflection waveguide using an on-chip electrically-pumped quantum dot laser

A. Schlager,<sup>1</sup> M. Götsch,<sup>1</sup> R. J. Chapman,<sup>1,2</sup> S. Frick,<sup>1</sup> H. Thiel,<sup>1</sup> H. Suchomel,<sup>3</sup> M. Kamp,<sup>3</sup> S. Höfling,<sup>3,4</sup> C. Schneider,<sup>3,5</sup> and G. Weihs<sup>1</sup>

<sup>1</sup>*Institut für Experimentalphysik, Universität Innsbruck, Technikerstraße 25, 6020 Innsbruck, Austria*

<sup>2</sup>*Quantum Photonics Laboratory and Centre for Quantum Computation and Communication Technology, School of Engineering, RMIT University, Melbourne, Victoria 3000, Australia*

<sup>3</sup>*Technische Physik, Universität Würzburg, Am Hubland, 97074 Würzburg, Germany*

<sup>4</sup>*School of Physics & Astronomy, University of St Andrews, St Andrews KY16 9SS, UK*

<sup>5</sup>*Institute of Physics, University of Oldenburg, D-26129 Oldenburg, Germany*

(Dated: July 14, 2021)

## 1. Calculating the effective nonlinearity

Using COMSOL Multiphysics<sup>®</sup> [1], we simulate the total internal reflection (T) modes at  $\sim 1580$  nm and the Bragg (B) mode at  $\sim 790$  nm for both polarizations (TE/TM). We can calculate the effective nonlinearity (at degeneracy) via

$$d_{\text{eff}} = \frac{\iint (E_B^{\text{TE}})^* d(x, y) E_T^{\text{TE}} E_T^{\text{TM}} dx dy}{\iint (E_B^{\text{TE}})^* E_T^{\text{TE}} E_T^{\text{TM}} dx dy}, \quad (\text{A1})$$

where  $d(x, y)$  is the spatial distribution of the nonlinear coefficients, which is dependent on the aluminum concentrations within our structure for a specific wavelength. The values for  $\text{Al}_x\text{Ga}_{1-x}\text{As}$  have been extracted from empiric data in Ref. [2] on pages 29-31.

## 2. Waveguide structure

In Fig. A1 scanning electron microscopy (SEM) images of our waveguide can be seen. One can also clearly discern a weakpoint of the gold layer at the intersection of the waveguide and BCB. Manufacturing restrictions deliver a possible reason as to why the gold does not withstand DC operation, as the temperature transport is disrupted and the heat spreads to a much smaller volume.

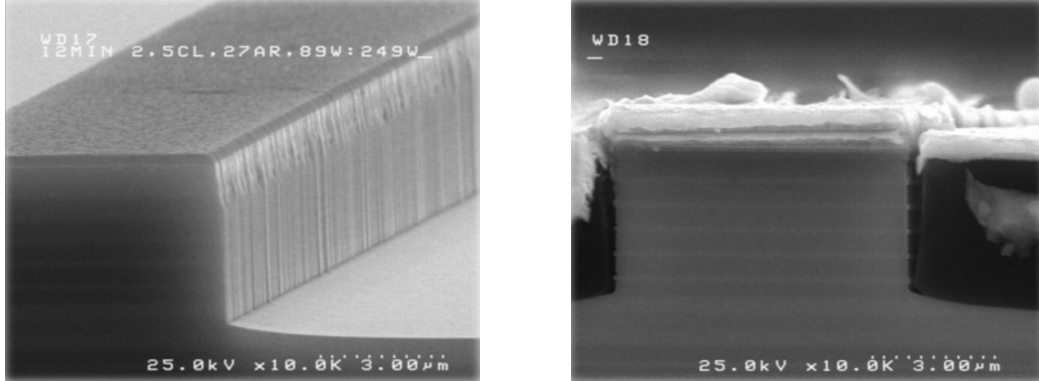

FIG. A1. SEM images of our BRW. On the left side, the waveguide ridge can be seen – the layers are visible on the facet. On the right side, the gold has been deposited on top of the waveguide and BCB.

### 3. Setup used for SHG and laser characterization

The setup used to characterize the internal laser and the second harmonic generation (SHG) within our BRWs is shown in Fig. A2. During the measurements either the telecom laser or the electric pulse generator was turned off, respectively.

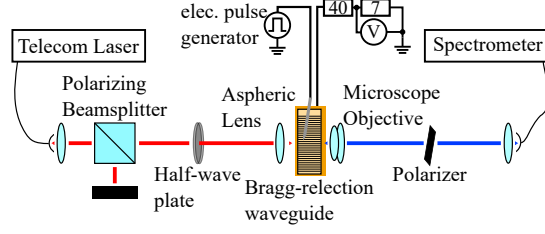

FIG. A2. Experimental setup for characterizing the internal QD laser and SHG spectra. We measure the SHG with the spectrometer by using the telecom laser and collecting the generated photons via the microscope objective. We explore all three types of SHG by adjusting the half-wave plate and polarizer settings. By turning on the electric pulse generator instead, we investigate the properties of the internal QD laser. We determine the peak currents by measuring the voltage with an oscilloscope at a  $7\ \Omega$  series resistance.

### 4. Temperature tuning

In order to find a temperature at which the phase-matching can occur, we analyze the laser and SHG spectrum. In Fig. A3a) we plot the laser spectrum versus temperature from  $0^\circ\text{C}$  to  $10^\circ\text{C}$  which enables tuning from 789 nm to 793 nm. The large spectral jumps of  $\sim 2\text{ nm}$  have been observed previously [3] and are caused by saturable absorption within AlGaAs laser structures [4, 5]. We then investigate the SHG spectrum for each type of nonlinear process by scanning the telecom laser wavelength and controlling the input and output polarization with half-wave plates and polarizers. We also use temperature to tune the phase-matching wavelength and plot the recorded central up-converted wavelengths in Fig. A3b). Our BRWs exclusively produce horizontally polarized output by type-2 SHG, which means the QD laser can only pump the corresponding DFG process. We find a working point for electrically pumped operation at  $3.5^\circ\text{C}$ , at which the spectra of the laser and type-2 process overlap, as can be seen in Figs. A3c) and d). The spectrum of the laser can be slightly tuned by fine adjustment of the temperature and current. This way, we are able to shift the intensity maximum from 791 nm to 792.9 nm, as shown in Fig. A3c). However, increasing the current by more than a few mA causes the central wavelength of the laser to shift away from the phase-matching wavelength. Therefore, we can only operate in a low-current regime and access  $\sim 8\ \mu\text{W}$  of normalized internal laser power while maintaining the high spectral overlap. Adjusting the phase-matching wavelength or laser spectrum by a few nanometers in future structures, by modifying the layer thicknesses or QD composition, could enable at least a tenfold increase in the usable laser power.

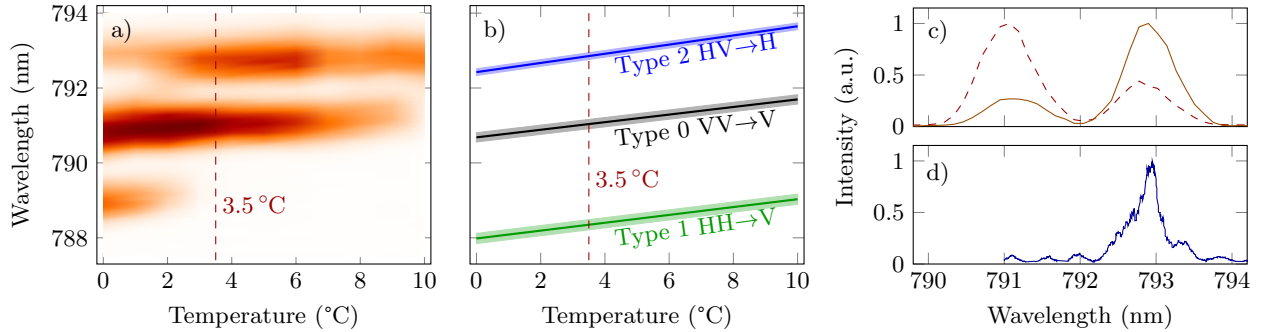

FIG. A3. a) Temperature dependence of the internal QD laser spectrum. b) Temperature dependence of the type-0 (black), type-1 (green) and type-2 (blue) SHG signal – the types are defined by the combination of horizontal (H) or vertical (V) polarization of the involved fields. The thick lines are linear fits of the measured central wavelengths and the bands indicate their standard deviation. c) Spectra of the internal laser at  $3.5^\circ\text{C}$  with two slightly different driving (peak) currents around 700 mA. The dashed line corresponds to the spectrum in a) and the solid line to a spectrum optimized for DFG. d) The type-2 second-harmonic-generation signal with its peak at 792.9 nm.

### 5. Correction of the laser powers

We measure the optical power of the external pump and seed laser in front of the objective and the internal pump power after the aspheric lens (see Fig. 3a) in the main text). Hence, we need to correct these values to get the normalized laser powers within the sample. This includes modelling the objective, facet reflections, the internal waveguide loss and the aspheric lens. Furthermore, the pump and seed lasers cannot be focused equally well by the microscope objective because of chromatic aberration, leading to reduced coupling efficiency into the waveguide for the external pump, as we optimize for the seed. As the spectrum of the internal pump is multi-modal, a part of its power is not phase-matched and is deducted as well. We measure 20 mW for the external pump before the objective and and 2.8  $\mu$ W internal pump after the aspheric lens, respectively. During the JSI measurement, the seed laser power is fixed to 10 mW. The losses for the external pump and seed laser are summarized Tab. A1. The effective power used in our efficiency calculations are adjusted by those amounts.

TABLE A1. Correction factors for the normalized laser powers.

|                                | External  | Seed      | Internal      |
|--------------------------------|-----------|-----------|---------------|
| Measured power                 | 20 mW     | 10 mW     | 2.8 $\mu$ W   |
| Objective                      | -1.487 dB | -5.850 dB | -             |
| Facet reflection               | -1.675 dB | -1.675 dB | +1.675 dB     |
| Average power in the waveguide | -2.545 dB | -2.890 dB | -2.242 dB     |
| Aspheric lens                  | -         | -         | +1.675 dB     |
| Coupling efficiency            | -3.000 dB | -         | -             |
| Spectral overlap               | -         | -         | -1.410 dB     |
| Normalized power               | 2.687 mW  | 0.909 mW  | 2.436 $\mu$ W |

This includes the propagation loss of our 1.48 mm long waveguide sample, which is -3.856 dB/mm at 790 nm and -4.458 dB/mm at 1620 nm. However, we are not interested in the total loss, but the average power within the device. Thus, we define how much of the laser light can actually be utilized within the waveguide via the Beer-Lambert-Law. The probability of photons reaching position  $z$  is

$$P_p(z) = 10^{-0.3856 \cdot z} \quad (\text{A2})$$

$$P_s(z) = 10^{-0.4458 \cdot z} \quad (\text{A3})$$

for the pump (p) and seed (s) laser. By integration we can estimate the average amount of light in the waveguide as

$$\bar{P}_{p/s} = \int_0^L \frac{P_{p/s}(z)}{L} dz, \quad (\text{A4})$$

which yields -2.545 dB and -2.89 dB for the external pump and seed laser, respectively. The internal laser needs to be in equilibrium, i.e. it needs to gain whatever power is lost at the facet within one trip. Thus, we can use the Beer-Lambert-Law again, and assume that the laser loses 68 % of its power at the facet (assuming no loss in the cavity, as it is offset by the gain). This way, we can estimate the average power of the internal laser within the device (in one direction) to be -2.242 dB in comparison to the total power at the facet.

## 6. Conversion efficiency correction

To be able to compare our results to similar structures, we have to correct the conversion efficiency for losses caused by the experimental setup, which are listed in Tab. A2. The idler photons experience the waveguide loss, get collected by the aspheric lens and pass through the polarization control and filters. All elements are coated for optimal transmission in the telecom wavelength range. Nonetheless, only  $-1.55$  dB of the light reaches the bandpass filter. The filter is centered at  $1540$  nm with a bandwidth of  $40$  nm and its transmission at the generated wavelengths is  $-1.25$  dB. After passing the filter, the light is coupled into a polarization maintaining single mode fiber. Due to the shape of the TIR mode, only about  $-5.23$  dB of the light can be coupled into the fiber. We include all fiber mating, spectrometer and camera losses, as well as the number of photons needed to produce a click in the detection efficiency  $\eta_{\text{det}} = -43.8$  dB of the InGaAs line camera, which is cooled to  $-80^\circ\text{C}$  to reduce noise.

TABLE A2. Overview of the correction factors used to determine the conversion efficiency. These values differ only very slightly for the various wavelengths used in the experiments.

|                                          | Losses (dB) |
|------------------------------------------|-------------|
| Waveguide losses                         | $-2.89$     |
| Aspheric lens (telecom)                  | $-0.22$     |
| Bandpass filter                          | $-1.25$     |
| Other Optics                             | $-1.55$     |
| Fiber-Coupling                           | $-5.23$     |
| Detection efficiency $\eta_{\text{det}}$ | $-43.80$    |
| Total loss                               | $-54.94$    |

## 7. Further DFG results

In addition to the previously shown data, we record the conversion efficiency of our active samples at different seed laser wavelengths, as can be seen in Tab. A3. The results show that our BRWs allow for consistent frequency conversion with a wavelength range of at least  $20$  nm. Analyzing the recorded joint spectral intensity, we expect this regime to be at least  $80$  nm wide. However, to access the DFG light near the degeneracy, the broad bandpass filter would have to be exchanged by a narrow and tunable one.

TABLE A3. Conversion efficiencies for different measurement settings, using the external and internal laser.

| type           | $\lambda_p$ | $\lambda_s$ (nm) | $\lambda_i$ (nm) | b (Hz/mW)                     | $\eta_{\text{conv}}(\%/W/\text{cm}^2)$ |
|----------------|-------------|------------------|------------------|-------------------------------|----------------------------------------|
| internal laser | 792.9       | 1607             | 1565             | $2.32 \pm 1.44$               | $0.26 \pm 0.17$                        |
|                |             | 1614             | 1558             | $3.56 \pm 1.44$               | $0.39 \pm 0.17$                        |
|                |             | 1619             | 1554             | $1.75 \pm 1.58$               | $0.19 \pm 0.18$                        |
|                |             | 1626             | 1548             | $5.70 \pm 1.55$               | $0.64 \pm 0.21$                        |
| external laser | 792.9       | 1607             | 1565             | $136 \pm 7$                   | $0.014 \pm 0.002$                      |
|                |             | 1614             | 1558             | $351 \pm 8$                   | $0.035 \pm 0.006$                      |
|                |             | 1619             | 1554             | $409 \pm 8$                   | $0.041 \pm 0.006$                      |
|                |             | 1626             | 1548             | $357 \pm 8$                   | $0.037 \pm 0.006$                      |
| passive sample | 767.3       | 1510             | 1560             | $(12.34 \pm 0.02) \cdot 10^3$ | $0.72 \pm 0.12$                        |

## REFERENCES

- 
- [1] COMSOL Multiphysics<sup>®</sup> v. 5.6. [www.comsol.com](http://www.comsol.com). COMSOL AB, Stockholm, Sweden.
  - [2] T. Günthner, “Classical and Nonclassical Optical Characterization of Bragg-Reflection Waveguides,” Ph.D. thesis, University of Innsbruck (2018).
  - [3] C. Autebert, G. Maltese, Y. Halioua, F. Boitier, A. Lemaître, M. Amanti, C. Sirtori, and S. Ducci, “Electrically Injected Twin Photon Emitting Lasers at Room Temperature,” *Technologies* **4**, 24 (2016), doi:10.3390/technologies4030024.
  - [4] J. Copeland, “Single-mode stabilization by traps in semiconductor lasers,” *IEEE Journal of Quantum Electronics* **16**, 721–727 (1980), doi:10.1109/JQE.1980.1070571.
  - [5] N. Chinone, T. Kuroda, T. Ohtoshi, T. Takahashi, and T. Kajimura, “Mode-hopping noise in index-guided semiconductor lasers and its reduction by saturable absorbers,” *IEEE Journal of Quantum Electronics* **21**, 1264–1270 (1985), doi:10.1109/JQE.1985.1072788.
